# Supplementary material for: Nonlinear Enhancement of Measurement Precision via a Hybrid Quantum Switch
Source: arXiv:2506.20632 source file (2025-06-25)
Supplement: Supplementary file 1 [file supplementary_material.pdf]

# Supplementary Material: Nonlinear Enhancement of Measurement Precision via a Hybrid Quantum Switch

## I. CALCULATION OF GENERATORS FOR CONVENTIONAL AND ICO SCHEMES

In quantum metrology, measurement protocols generally follow a definite causal order. Take a conventional process as an example, where orbital angular momentum (OAM) shifting is performed first, followed by rotation. This process is represented as $U_\theta^{(m)} = (D_{2\theta})^m D_{2l\hbar}$. The generator of the entire process can be derived as follows:

$$\begin{aligned} h_{MP} &= i[\partial_\theta U_c]U_c^\dagger \\ &= i[\partial_\theta D_{2m\theta}]D_{2m\theta}^\dagger \\ &= \frac{2m\hat{L}_z}{\hbar}. \end{aligned} \tag{1}$$

Subsequently, the precision of parameter estimation can be obtained through this generator, expressed as $\delta\theta_c \geq \frac{1}{4m\Delta L_z}$. In this bound, the precision is determined by the variance of $\hat{L}_z$ in the probe state.

In the quantum switch protocol, the system's evolution is governed by the unitary operator $W_{QS} = (D_{2\hbar})^l (D_{2\theta})^m \otimes |0\rangle\langle 0| + (D_{2\theta})^m (D_{2\hbar})^l \otimes |1\rangle\langle 1|$, where the $m$ and $l$ is the number of query times of evolution process. The corresponding generator within the ICO process can be formally expressed as:

$$\begin{aligned} h_{QS} &= i[\partial_\theta W_{QS}]W_{QS}^\dagger \\ &= \frac{2m}{\hbar}\left[\hat{L}_z \otimes |0\rangle\langle 0| + D_{2l\hbar}\hat{L}_z D_{2l\hbar}^\dagger \otimes |1\rangle\langle 1|\right] \\ &= 2m(\frac{\hat{L}_z}{\hbar} + l) - 2ml\hat{\sigma_z}. \end{aligned} \tag{2}$$

Under this framework, the control qubits are initialized in the superposition state $\frac{1}{2}(|0\rangle + |1\rangle)$, which remains fixed throughout the protocol. The resultant precision scaling is quantified by the bound $\delta\theta \geq \frac{1}{4m\Delta L_z/\hbar + 4ml}$. The generator of the quantum switch protocol, characterized by $\Delta h_{QS} = 2m\frac{\Delta \hat{L}_z}{\hbar} + 2ml$, introduces a fundamental distinction from conventional quantum metrology paradigms. Notably, the emergence of the additional term $2ml$, arising from coherent control of gate order, demonstrates that the intrinsic uncertainty inherent in the process constitutes a non-negligible contribution to the final precision limit.

## II. NECESSITY OF THE HOLLOW ROOF PRISM

Unlike the usual usage of the hollow roof prism (HRP) to introduce an optical delay, the beam shining on the HRP is centering around the Dihedral Line (Roof Joint) so the reflected beam exactly overlaps with the incident beam. The Dihedral Line inevitably causes single-slit diffraction, which can be spatially filtered by the pinhole.

The HRP meanwhile reverses wavevector $k$ and reflects the $y$ coordinate, and its operator $\Pi$ can be defined via $\Pi|x\rangle \otimes |y\rangle \otimes |k\rangle = |x\rangle \otimes |-y\rangle \otimes |-k\rangle$. One horizontally placed Dove prism merely reflects the $y$ coordinate of a photon and can be expressed as $P|x\rangle \otimes |y\rangle \otimes |k\rangle = |x\rangle \otimes |-y\rangle \otimes |k\rangle$; and rotating the Dove prism by an angle of $\theta$, the operation becomes $P_\theta = R^\dagger(\theta)PR(\theta)$. The action of a pair of Dove prisms on the forth and back way can be written as $PP_\theta = R(2\theta)$ and $P_\theta P = R^\dagger(2\theta)$ respectively. Thus, a round trip consisting of $m/2$ ($m$ is an even number) pairs of Dove prisms and one HRP eventually rotates the photon by $2m\theta$, since we have

$$R^\dagger(m\theta)\Pi R(m\theta) = \Pi R(2m\theta). \tag{3}$$

In contrast, a normal mirror acts as $R^\dagger(2\theta)R(2\theta) = I$ and fails to encode the parameter to be measured.

## III. FISHER INFORMATION CALCULATION

The geometric phase imposed on the control qubit in the state $(|0\rangle + |1\rangle)$ renders a pointer for measuring $\theta$, and the extractable Fisher information by measuring this phase is proportional to $m \cdot l$. When we input a state $(|0\rangle + |1\rangle) \otimes |\Phi_i\rangle$, the output state after all the quantum SWITCH is written as:

$$\begin{aligned} &|\Psi_f\rangle = (D_{l\hbar}^\dagger D_{2m\theta} D_{l\hbar}|0\rangle + D_{l\hbar} D_{2m\theta} D_{l\hbar}^\dagger |1\rangle) \otimes |\Phi_i\rangle \\ &= (e^{-i2ml\theta}|0\rangle + e^{i2ml\theta}|1\rangle) \otimes D_{m\theta}|\Phi_i\rangle \\ &= |\varphi_f\rangle \otimes |\Phi_f\rangle \end{aligned} \tag{4}$$

where $|\psi_f\rangle$ is the output state of the pointer, and $|\Phi_i\rangle$ and $|\Phi_f\rangle$ are the initial and final state of the system. Then, a direct calculation of quantum Fisher information(QFI) is given by [1, 2]:

$$Q_\theta = 4(\langle \partial_\theta \Psi_f | \partial_\theta \Psi_f\rangle - \langle \partial_\theta \Psi_f | \Psi_f\rangle\langle \Psi_f | \partial_\theta \Psi_f\rangle) \tag{5}$$

Here, we have the derivation $|\partial_\theta \Psi_f\rangle = |\partial_\theta \varphi_f\rangle \otimes |\Phi_f\rangle + |\varphi_f\rangle \otimes |\partial_\theta \Phi_f\rangle$. Thus, the quantum Fisher information can be divided into two parts:

$$Q_\theta = Q_\theta^p + Q_\theta^s. \tag{6}$$

The first term is calculated as $Q_\theta^p = 16m^2l^2$ and can be extracted by measuring the pointer state. The second term $Q_\theta^s$ represents the QFI of the system state which is related to the final distribution of photon transverse mode. In the sense that the transverse mode is discarded

in the final measurement, the specific form of $Q^s_\theta$ is not of interest here.

To saturate the QFI, we project the pointer to $|\pm\rangle$ and the theoretical probabilities calculates as $P_\pm(\theta) = \frac{1}{2}[1 \pm \cos(4ml\theta)]$. The extracted Fisher information(FI) is then given by

$$F^p_\theta = \frac{1}{P_+(\theta)}\left[\frac{\partial P_+(\theta)}{\partial\theta}\right]^2 + \frac{1}{P_-(\theta)}\left[\frac{\partial P_-(\theta)}{\partial\theta}\right]^2 = 16m^2l^2 \tag{7}$$

From the Cramer-Rao bound, the RMSE to estimate $\theta$ satisfies

$$\delta\theta \geq \frac{1}{\sqrt{\nu F_\theta}} = \frac{1}{4\sqrt{\nu}ml} \tag{8}$$

which indicates that the nonlinear enhanced precision can be attained by the projective measurement on the control qubit.

The nonlinear precision enhancement cannot be achieved solely through the OAM shifting operation without coherent control of gate order. When considering that an $l$-order OAM state is generated by an OAM shifting followed by an unknown rotation, the state after applying fixed-order gates can be expressed as

$$\begin{aligned} Q_\theta(|\psi_{\text{fixed}}\rangle) &= 4|\langle +l|(\partial_\theta D_{2m\theta})(\partial_\theta D^\dagger_{2m\theta})|+l\rangle \\ &\quad - 4|\langle +l|\partial_\theta D^\dagger_{2m\theta}|+l\rangle|^2 \\ &= 4\cdot(4m^2l^2) - 4\cdot(2ml)^2 \\ &= 0. \end{aligned} \tag{9}$$

The result of zero quantum Fisher information indicates that no information regarding $\theta$ can be extracted in this fixed process. This outcome is readily understandable, as the rotational transformation applied to the OAM eigenstate introduces an additional global phase factor that is not directly observable. It is also important to note that in our experiment, $l$ refers to the order of the OAM shift gate rather than the order of OAM eigenstates; thus, any arbitrary input system state will consistently map to the same measurement result.

Considering an alternative experimental configuration of the Mach-Zehnder (MZ) interferometer [3], a photon is prepared in a superposition of two paths. In this setup, one path undergoes a rotation operation while the other remains unchanged. The process can be described by the expression $D_{2m\theta}|0\rangle\langle 0| + |1\rangle\langle 1|$. Starting with an initial state $|+l\rangle$ and employing the path state $\frac{1}{\sqrt{2}}(|0\rangle + |1\rangle)$, the joint state of the system and path after applying the rotation operation can be expressed as

$$|\Phi_f\rangle = \frac{1}{\sqrt{2}}(D_{2m\theta}|+l\rangle|0\rangle + |+l\rangle|1\rangle). \tag{10}$$

Then, the QFI is calculated via Eq. 5 as

$$Q_\theta(\Phi_f) = 4\left(2m^2l^2\theta^2 - |\frac{1}{2}i2ml\theta|^2\right) = 4m^2l^2\theta^2, \tag{11}$$

where it is noted that the QFI for this MZ interference configuration is only one quarter of that obtained from a quantum switch configuration. Furthermore, it should be emphasized that the visibility of Mach-Zehnder (MZ) interferometry is limited by the rotational symmetry inherent in the input beam distribution; thus, theoretically calculated QFI cannot be fully realized under conditions of imperfect state preparation.

## VI. THE JONES MATRIX OF DOVE PRISM

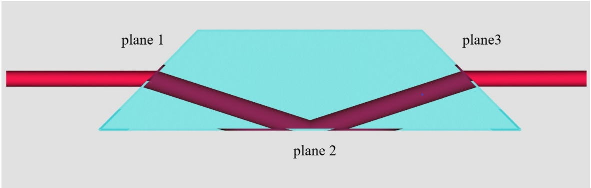


FIG. 1. **Photon transmission through horizontally placed Dove prism**. The incident photon is refracted at plane1 and then totally reflected at the inner plane2, and finally exits the prism after being refracted at plane3.

The photon propagating through a Dove prism experiences twice refraction on the incident and exit planes (labeled as plane1 and 3 in Fig. (1), and one time of total inner reflection on the bottom plane (labeled as plane2 in Fig. (1). Both photon loss and polarization alteration occur during the transmission of a Dove prism, which cannot be represented by a unitary transformation. An alternative way to describe this process is using the Jones matrix which can be derived from Finel formulas. When the Dove prism is horizontally placed, the Jones matrix can be written as:

$$J(0) = \begin{bmatrix} t^s_3 r^s_2 t^s_1 & 0 \\ 0 & t^p_3 r^p_2 t^p_1 \end{bmatrix}, \tag{12}$$

in which $t^{s/p}_i (r^{s/p}_i)$ represents the transmission (reflection) coefficient of $s/p$ wave on the $i_{th}$ plane. When Dove prism is rotated by an angle $\theta$, the Jones matrix changes to[4]:

$$\begin{aligned} J(\theta) &= R^\dagger(\theta)J(0)R(\theta) \\ &= \begin{bmatrix} \tau_s\cos^2\theta + \tau_p\sin^2\theta & (\tau_s - \tau_p)\cos\theta\sin\theta \\ (\tau_p - \tau_s)\cos\theta\sin\theta & \tau_s\sin^2\theta + \tau_p\cos^2\theta \end{bmatrix}, \end{aligned} \tag{13}$$

where $\tau_s$ and $\tau_p$ stand for $t_{3s}r_{2s}t_{1s}$ and $t_{3p}r_{2p}t_{1p}$ respectively and $R(\theta)$ is the SO(2) rotation matrix. Then, we find the conclusion that $J(\theta)\cdot J(\theta + \frac{\pi}{2}) \propto I$ from the expression of $J(\theta)$ in Eq. (12).

[1] Helstrom, C. W. Quantum detection and estimation theory. Journal of Statistical Physics. *Journal of Statistical Physics* **1**, 231–252 (1969).
[2] Holevo, A. S. *Probabilistic and statistical aspects of quantum theory*, vol. 1 (Springer Science & Business Media, 2011).
[3] Courtial, J., Dholakia, K., Robertson, D., Allen, L. & Padgett, M Measurement of the rotational frequency shift imparted to a rotating light beam possessing orbital angular momentum. *Physical review letters* **80**, 3217 (1998).
[4] Moreno, I. Jones matrix for image-rotation prisms. *Applied Optics* **43**, 3373–3381 (2004).
